# Supplementary material for: TinyLidarNet: 2D LiDAR-based End-to-End Deep Learning Model for F1TENTH Autonomous Racing
Source: arXiv:2410.07447 source file (2024-10-09)
Supplement: Supplementary file 1 [file appendix.tex]

\appendix
\section{Appendix A: Additional Stuff}\label{sec:acknowledge}
